# Supplementary material for: Cure Rate Joint Model for Time-to-Event Data and Longitudinal Tumor Burden with Potential Change Points
Source: arXiv:2507.18773 source file (2025-07-24)
Supplement: Supplementary file 1 [file supp.pdf]

# Supplementary Notes for “Cure Rate Joint Model for Time-to-Event Data and Longitudinal Tumor Burden with Potential Change Points”

## Contents

|          |                                                                                                         |           |
|----------|---------------------------------------------------------------------------------------------------------|-----------|
| <b>1</b> | <b>Details for Q function</b>                                                                           | <b>2</b>  |
| 1.1      | Full Q function . . . . .                                                                               | 2         |
| 1.2      | Decomposition of the Q function . . . . .                                                               | 2         |
| <b>2</b> | <b>Details for the E-step</b>                                                                           | <b>3</b>  |
| 2.1      | Properties of the longitudinal outcome for the individuals in the change-point group . . . . .          | 3         |
| 2.2      | Further details for the E-step related to $Q^{(1)}$ . . . . .                                           | 4         |
| 2.3      | Further details for the E-step related to $Q^{(2)}$ . . . . .                                           | 4         |
| 2.4      | Further details for the E-step related to $Q^{(3)}$ . . . . .                                           | 5         |
| 2.5      | Further details for the E-step related to $Q^{(4)}$ . . . . .                                           | 5         |
| <b>3</b> | <b>Details for the M-steps</b>                                                                          | <b>6</b>  |
| 3.1      | Closed-form solutions for some parameters in the M-step . . . . .                                       | 6         |
| 3.2      | Closed-form solutions for some parameters in the M-step in scalar form . . . . .                        | 7         |
| 3.3      | The derivative of Q function with respect to $\boldsymbol{\mu}_r$ and $\boldsymbol{\Sigma}_r$ . . . . . | 8         |
| 3.3.1    | Calculation of $\frac{\partial Q}{\partial \boldsymbol{\mu}_r}$ . . . . .                               | 8         |
| 3.3.2    | Calculation of $\frac{\partial Q}{\partial \text{vech}(\boldsymbol{P}_r)}$ . . . . .                    | 9         |
| <b>4</b> | <b>Details for the longitudinal trajectory estimations</b>                                              | <b>10</b> |
| 4.1      | The derivation for the longitudinal trajectory estimations . . . . .                                    | 10        |
| 4.2      | Monte Carlo sampling for the longitudinal trajectory estimations . . . . .                              | 10        |
| <b>5</b> | <b>Details in simulation</b>                                                                            | <b>11</b> |
| 5.1      | The parameters used in the simulation . . . . .                                                         | 11        |
| 5.2      | Other simulation results . . . . .                                                                      | 11        |
| <b>6</b> | <b>The overall estimations of the parameters in the EMPOWER study</b>                                   | <b>11</b> |
| 6.1      | Overall change point, pre- and post-slope calculation . . . . .                                         | 11        |
| 6.2      | The overall estimations in the EMPOWER study . . . . .                                                  | 14        |
| <b>7</b> | <b>Proofs</b>                                                                                           | <b>14</b> |

# 1 Details for Q function

## 1.1 Full Q function

The Q-function for this paper is shown as (1).

$Q = \text{Constant}$

$$\begin{aligned}
& + \sum_{i=1}^n \left( \nu_i \log(1 - \pi_{(s)}) + (1 - \nu_i) E[\Delta_i | t_i^* > t_i, \mathbf{y}_i] \log(\pi_{(s)}) + (1 - \nu_i) E[1 - \Delta_i | t_i^* > t_i, \mathbf{y}_i] \log(1 - \pi_{(s)}) \right) \\
& + \sum_{i=1}^n \nu_i \left( -\frac{1}{2} \log(\sigma_{tte}^2) - \frac{(t_i - \mathbf{X}_{tte,i}^T \boldsymbol{\gamma})^2}{2\sigma_{tte}^2} \right) \\
& + \sum_{i=1}^n \nu_i \left( -\frac{1}{2} \log(|\boldsymbol{\Sigma}_r|) - \frac{1}{2} E[(\mathbf{r}_i - \boldsymbol{\mu}_r)^T \boldsymbol{\Sigma}_r^{-1} (\mathbf{r}_i - \boldsymbol{\mu}_r) | t_i^* = t_i, \mathbf{y}_i, \Delta_i = 0] \right) \\
& + \sum_{i=1}^n \nu_i \left( -\log \left( \Phi \left( \frac{e^{t_i} - \mu_\omega}{\sigma_\omega} \right) - \Phi \left( \frac{-\mu_\omega}{\sigma_\omega} \right) \right) \right) \\
& + \sum_{i=1}^n \nu_i \left( -\frac{n_i}{2} \log(\sigma_y^2) - \frac{E[\|\mathbf{y}_i - \mathbf{Z}_i \mathbf{b}_i - \mathbf{X}_i \boldsymbol{\beta}\|_2^2 | t_i^* = t_i, \mathbf{y}_i, \Delta_i = 0]}{2\sigma_y^2} \right) \\
& + \sum_{i=1}^n (1 - \nu_i) E[1 - \Delta_i | t_i^* > t_i, \mathbf{y}_i] \left( -\frac{1}{2} \log(\sigma_{tte}^2) - \frac{E[(t_i^* - \mathbf{X}_{tte,i}^T \boldsymbol{\gamma})^2 | t_i^* > t_i, \mathbf{y}_i, \Delta_i = 0]}{2\sigma_{tte}^2} \right) \\
& + \sum_{i=1}^n (1 - \nu_i) E[1 - \Delta_i | t_i^* > t_i, \mathbf{y}_i] \left( -\frac{1}{2} \log(|\boldsymbol{\Sigma}_r|) - \frac{1}{2} E[(\mathbf{r}_i - \boldsymbol{\mu}_r)^T \boldsymbol{\Sigma}_r^{-1} (\mathbf{r}_i - \boldsymbol{\mu}_r) | t_i^* > t_i, \mathbf{y}_i, \Delta_i = 0] \right) \\
& + \sum_{i=1}^n (1 - \nu_i) E[1 - \Delta_i | t_i^* > t_i, \mathbf{y}_i] \left( -E \left[ \log \left( \Phi \left( \frac{e^{t_i^*} - \mu_\omega}{\sigma_\omega} \right) - \Phi \left( \frac{-\mu_\omega}{\sigma_\omega} \right) \right) | t_i^* > t_i, \mathbf{y}_i, \Delta_i = 0 \right] \right) \\
& + \sum_{i=1}^n (1 - \nu_i) E[1 - \Delta_i | t_i^* > t_i, \mathbf{y}_i] \left( -\frac{n_i}{2} \log(\sigma_y^2) - \frac{E[\|\mathbf{y}_i - \mathbf{Z}_i \mathbf{b}_i - \mathbf{X}_i \boldsymbol{\beta}\|_2^2 | t_i^* > t_i, \mathbf{y}_i, \Delta_i = 0]}{2\sigma_y^2} \right) \\
& + \sum_{i=1}^n (1 - \nu_i) E[\Delta_i | t_i^* > t_i, \mathbf{y}_i] \left( -\frac{1}{2} \log(|\boldsymbol{\Sigma}_{r,(s)}|) - \frac{1}{2} E[(\mathbf{b}_{(s),i} - \boldsymbol{\mu}_{r,(s)})^T \boldsymbol{\Sigma}_{r,(s)}^{-1} (\mathbf{b}_{(s),i} - \boldsymbol{\mu}_{r,(s)}) | \mathbf{y}_i, \Delta_i = 1] \right) \\
& + \sum_{i=1}^n (1 - \nu_i) E[\Delta_i | t_i^* > t_i, \mathbf{y}_i] \left( -\frac{n_i}{2} \log(\sigma_{y,(s)}^2) - \frac{E[\|\mathbf{y}_i - \mathbf{Z}_{(s),i} \mathbf{b}_{(s),i} - \mathbf{X}_{(s),i} \boldsymbol{\beta}_{(s)}\|_2^2 | \mathbf{y}_i, \Delta_i = 1]}{2\sigma_{y,(s)}^2} \right). \quad (1)
\end{aligned}$$

## 1.2 Decomposition of the Q function

We decompose the Q function into four components (ignoring the constant), i.e.,  $Q = Q^{(1)} + Q^{(2)} + Q^{(3)} + Q^{(4)}$ . And we list the four components explicitly as follows. To simplify our notation, we use subscript 0 or 1 to denote  $\Delta = 0$  or  $\Delta = 1$ , respectively, and we use superscript  $(=)$  or  $(>)$  to denote the situation where  $t_i^* = t_i$  or  $t_i^* > t_i$ . All expectations in this section are conditional on the observed data. In particular, we let  $E^{(=)}[A_i]$  denote  $E[A_i | t_i^* = t_i, \mathbf{y}_i]$ ,  $E^{(>)}[A_i]$  denote  $E[A_i | t_i^* > t_i, \mathbf{y}_i]$ ,  $E_0^{(=)}[A_i]$  denote  $E[A_i | t_i^* = t_i, \mathbf{y}_i, \Delta_i = 0]$ ,  $E_0^{(>)}[A_i]$  denote  $E[A_i | t_i^* > t_i, \mathbf{y}_i, \Delta_i = 0]$ , and  $E_1^{(>)}[A_i]$  denote  $E[A_i | t_i^* > t_i, \mathbf{y}_i, \Delta_i = 1]$ .

$Q^{(1)}$  includes the terms related to the parameter  $\pi_{(s)}$ , i.e.,

$$Q^{(1)} = \sum_{i=1}^n \left( \nu_i \log(1 - \pi_{(s)}) + (1 - \nu_i) E^{(>)}[\Delta_i] \log(\pi_{(s)}) + (1 - \nu_i) E^{(>)}[1 - \Delta_i] \log(1 - \pi_{(s)}) \right).$$

$Q^{(2)}$  includes the terms representing those subjects whose event times are observed, i.e.,

$$\begin{aligned} Q^{(2)} = & \sum_{i=1}^n \nu_i \left( -\frac{1}{2} \log(\sigma_{tte}^2) - \frac{(t_i - \mathbf{w}_i^T \boldsymbol{\gamma})^2}{2\sigma_{tte}^2} \right) \\ & + \sum_{i=1}^n \nu_i \left( -\frac{1}{2} \log(|\boldsymbol{\Sigma}_r|) - \frac{1}{2} E_0^{(=)}[(\mathbf{r}_i - \boldsymbol{\mu}_r)^T \boldsymbol{\Sigma}_r^{-1} (\mathbf{r}_i - \boldsymbol{\mu}_r)] \right) \\ & + \sum_{i=1}^n \nu_i \left( -\log \left( \Phi \left( \frac{e^{t_i} - \mu_\omega}{\sigma_\omega} \right) - \Phi \left( \frac{-\mu_\omega}{\sigma_\omega} \right) \right) \right) \\ & + \sum_{i=1}^n \nu_i \left( -\frac{n_i}{2} \log(\sigma_y^2) - \frac{E_0^{(=)}[\|\mathbf{y}_i - \mathbf{Z}_i \mathbf{b}_i - \mathbf{X}_i \boldsymbol{\beta}\|_2^2]}{2\sigma_y^2} \right). \end{aligned}$$

$Q^{(3)}$  includes the terms related to those who are censored and experience a change point, i.e.,

$$\begin{aligned} Q^{(3)} = & \sum_{i=1}^n (1 - \nu_i) E^{(>)}[1 - \Delta_i] \left( -\frac{1}{2} \log(\sigma_{tte}^2) - \frac{E_0^{(>)}[(t_i^* - \mathbf{w}_i^T \boldsymbol{\gamma})^2]}{2\sigma_{tte}^2} \right) \\ & + \sum_{i=1}^n (1 - \nu_i) E^{(>)}[1 - \Delta_i] \left( -\frac{1}{2} \log(|\boldsymbol{\Sigma}_r|) - \frac{1}{2} E_0^{(>)}[(\mathbf{r}_i - \boldsymbol{\mu}_r)^T \boldsymbol{\Sigma}_r^{-1} (\mathbf{r}_i - \boldsymbol{\mu}_r)] \right) \\ & + \sum_{i=1}^n (1 - \nu_i) E^{(>)}[1 - \Delta_i] \left( -E_0^{(>)} \left[ \log \left( \Phi \left( \frac{e^{t_i^*} - \mu_\omega}{\sigma_\omega} \right) - \Phi \left( \frac{-\mu_\omega}{\sigma_\omega} \right) \right) \right] \right) \\ & + \sum_{i=1}^n (1 - \nu_i) E^{(>)}[1 - \Delta_i] \left( -\frac{n_i}{2} \log(\sigma_y^2) - \frac{E_0^{(>)}[\|\mathbf{y}_i - \mathbf{Z}_i \mathbf{b}_i - \mathbf{X}_i \boldsymbol{\beta}\|_2^2]}{2\sigma_y^2} \right). \end{aligned}$$

$Q^{(4)}$  includes the terms related to those censored subjects who are not at risk of change points, i.e.,

$$\begin{aligned} Q^{(4)} = & \sum_{i=1}^n (1 - \nu_i) E^{(>)}[\Delta_i] \left( -\frac{1}{2} \log(|\boldsymbol{\Sigma}_{r,(s)}|) - \frac{1}{2} E_1[(\mathbf{b}_{(s),i} - \boldsymbol{\mu}_{r,(s)})^T \boldsymbol{\Sigma}_{r,(s)}^{-1} (\mathbf{b}_{(s),i} - \boldsymbol{\mu}_{r,(s)})] \right) \\ & + \sum_{i=1}^n (1 - \nu_i) E^{(>)}[\Delta_i] \left( -\frac{n_i}{2} \log(\sigma_{y,(s)}^2) - \frac{E_1[\|\mathbf{y}_i - \mathbf{Z}_{(s),i} \mathbf{b}_{(s),i} - \mathbf{X}_{(s),i} \boldsymbol{\beta}_{(s)}\|_2^2]}{2\sigma_{y,(s)}^2} \right). \end{aligned}$$

## 2 Details for the E-step

### 2.1 Properties of the longitudinal outcome for the individuals in the change-point group

Based on the derivation in [Alt et al., 2025], let  $\boldsymbol{\mu}_{b|\omega_i} = \boldsymbol{\mu}_b + \frac{\boldsymbol{\sigma}_{b\omega}}{\sigma_\omega^2}(\omega_i - \mu_\omega)$  and  $\boldsymbol{\Sigma}_{b|\omega} = \boldsymbol{\Sigma}_b - \frac{1}{\sigma_\omega^2} \boldsymbol{\sigma}_{b\omega} \boldsymbol{\sigma}_{b\omega}^T$ , we notice that

$$\begin{pmatrix} \mathbf{y}_i \\ \mathbf{b}_i \end{pmatrix} \bigg|_{\omega_i, \Delta_i = 0} \sim N_{n_i+3} \left( \begin{pmatrix} \boldsymbol{\mu}_{y|\omega_i} \\ \boldsymbol{\mu}_{b|\omega_i} \end{pmatrix}, \begin{pmatrix} \boldsymbol{\Sigma}_{y|\omega_i} & \boldsymbol{\Sigma}_{yb|\omega_i} \\ \boldsymbol{\Sigma}_{yb|\omega_i}^T & \boldsymbol{\Sigma}_{b|\omega_i} \end{pmatrix} \right),$$

where  $\boldsymbol{\mu}_{\mathbf{y}|\omega_i} = \mathbf{X}_i\boldsymbol{\beta} + \mathbf{Z}_i\boldsymbol{\mu}_{\mathbf{b}|\omega_i}$ ,  $\boldsymbol{\Sigma}_{\mathbf{y}|\omega_i} = \sigma_y^2\mathbf{I}_{n_i} + \mathbf{Z}_i\boldsymbol{\Sigma}_{\mathbf{b}|\omega_i}\mathbf{Z}_i^T$ , and  $\boldsymbol{\Sigma}_{\mathbf{y}\mathbf{b}|\omega_i} = \mathbf{Z}_i\boldsymbol{\Sigma}_{\mathbf{b}|\omega_i}$ . Hence, we have that  $\mathbf{y}_i|\omega_i, \Delta_i = 0 \sim N_{n_i}(\mathbf{X}_i\boldsymbol{\beta} + \mathbf{Z}_i\boldsymbol{\mu}_{\mathbf{b}|\omega_i}, \sigma_y^2\mathbf{I}_{n_i} + \mathbf{Z}_i\boldsymbol{\Sigma}_{\mathbf{b}|\omega_i}\mathbf{Z}_i^T)$ .

Using the properties of multivariate normal distribution, we have  $E[\mathbf{b}_i|\omega_i, \mathbf{y}_i, \Delta_i = 0] = \boldsymbol{\mu}_{\mathbf{b}|\omega_i} + \boldsymbol{\Sigma}_{\mathbf{y}\mathbf{b}|\omega_i}^T \boldsymbol{\Sigma}_{\mathbf{y}|\omega_i}^{-1} (\mathbf{y}_i - \boldsymbol{\mu}_{\mathbf{y}|\omega_i})$  and  $\text{Var}(\mathbf{b}_i|\omega_i, \mathbf{y}_i, \Delta_i = 0) = \boldsymbol{\Sigma}_{\mathbf{b}|\omega_i} - \boldsymbol{\Sigma}_{\mathbf{y}\mathbf{b}|\omega_i}^T \boldsymbol{\Sigma}_{\mathbf{y}|\omega_i}^{-1} \boldsymbol{\Sigma}_{\mathbf{y}\mathbf{b}|\omega_i}$ , and we can also get  $E[\mathbf{b}_i\mathbf{b}_i^T|\omega_i, \mathbf{y}_i, \Delta_i = 0] = E[\mathbf{b}_i|\omega_i, \mathbf{y}_i, \Delta_i = 0]E[\mathbf{b}_i|\omega_i, \mathbf{y}_i, \Delta_i = 0]^T + \text{Var}(\mathbf{b}_i|\omega_i, \mathbf{y}_i, \Delta_i = 0)$ .

## 2.2 Further details for the E-step related to $Q^{(1)}$

We first note that  $\mathbf{b}_{(s),i}|\Delta_i = 1 \sim N(\boldsymbol{\mu}_{r,(s)}, \boldsymbol{\Sigma}_{r,(s)})$  and  $\mathbf{y}_i|\mathbf{b}_{(s),i}, \Delta_i = 1 \sim N_{n_i}(\mathbf{X}_{(s),i}\boldsymbol{\beta}_{(s)} + \mathbf{Z}_{(s),i}\mathbf{b}_{(s),i}, \sigma_{y,(s)}^2\mathbf{I}_{n_i})$ . Using standard properties of multivariate normal distributions, we obtain

$$P(\mathbf{y}_i|\Delta_i = 1) = \phi\left(\mathbf{y}_i|\mathbf{X}_{(s),i}\boldsymbol{\beta}_{(s)} + \mathbf{Z}_{(s),i}\boldsymbol{\mu}_{r,(s)}, \sigma_{y,(s)}^2\mathbf{I}_{n_i} + \mathbf{Z}_{(s),i}\boldsymbol{\Sigma}_{r,(s)}\mathbf{Z}_{(s),i}^T\right).$$

Additionally,  $P(t_i^* > t_i, \mathbf{y}_i|\Delta_i = 0)$  may be computed as

$$\begin{aligned} P(t_i^* > t_i, \mathbf{y}_i|\Delta_i = 0) &= \int_{t_i}^{\infty} f(t_i^*, \mathbf{y}_i|\Delta_i = 0) dt_i^* \\ &= \int_{t_i}^{\infty} \int_0^{e^{t_i^*}} f(t_i^*, \mathbf{y}_i, \omega_i|\Delta_i = 0) d\omega_i dt_i^* \\ &= \int_{t_i}^{\infty} \int_0^{e^{t_i^*}} f(\mathbf{y}_i|\omega_i, \Delta_i = 0) f(\omega_i|t_i^*, \Delta_i = 0) f(t_i^*|\Delta_i = 0) d\omega_i dt_i^*. \end{aligned} \quad (2)$$

The Monte Carlo integration of (2) is provided in 2.4 (for the denominator).

## 2.3 Further details for the E-step related to $Q^{(2)}$

We aim to calculate (3), whose proof is provided in 7, and we propose to calculate the numerator and denominator separately. The denominator is a special case of the numerator when  $h_1$ ,  $h_2$ , and  $h_3$  are all equal to 1. Therefore, we only provide the procedure for the Monte Carlo integration of the numerator.

$$\begin{aligned} &E[h_1(t_i^*) \cdot h_2(\omega_i) \cdot h_3(\mathbf{b}_i)|t_i^* = t_i, \mathbf{y}_i, \Delta_i = 0] \\ &= \frac{\int_0^{e^{t_i^*}} h_1(t_i^*) \cdot h_2(\omega_i) E[h_3(\mathbf{b}_i)|\mathbf{y}_i, \omega_i, \Delta_i = 0] f(\mathbf{y}_i|\omega_i, \Delta_i = 0) f(\omega_i|t_i^*, \Delta_i = 0) d\omega_i}{\int_0^{e^{t_i^*}} f(\mathbf{y}_i|\omega_i, \Delta_i = 0) f(\omega_i|t_i^*, \Delta_i = 0) d\omega_i}. \end{aligned} \quad (3)$$

To calculate the numerator  $\int_0^{e^{t_i^*}} h_1(t_i^*) \cdot h_2(\omega_i) E[h_3(\mathbf{b}_i)|\mathbf{y}_i, \omega_i, \Delta_i = 0] f(\mathbf{y}_i|\omega_i, \Delta_i = 0) f(\omega_i|t_i^*, \Delta_i = 0) d\omega_i$ , the following procedure can be used. First, for  $j \in \{1, 2, \dots, J\}$ , sample  $\omega_i^{(j)} \sim TN(\mu_\omega, \sigma_\omega^2, 0, e^{t_i^*})$ . Then, the integral can be approximated using the Monte Carlo estimator  $\int_0^{e^{t_i^*}} h_1(t_i^*) \cdot h_2(\omega_i) E[h_3(\mathbf{b}_i)|\mathbf{y}_i, \omega_i, \Delta_i = 0] f(\mathbf{y}_i|\omega_i, \Delta_i = 0) f(\omega_i|t_i^*, \Delta_i = 0) d\omega_i \approx \frac{1}{J} \sum_{j=1}^J h_1(t_i^*) \cdot h_2(\omega_i^{(j)}) \cdot E[h_3(\mathbf{b}_i)|\mathbf{y}_i, \omega_i^{(j)}, \Delta_i = 0] \cdot f(\mathbf{y}_i|\omega_i^{(j)}, \Delta_i = 0)$ , where  $f(\mathbf{y}_i|\omega_i^{(j)}, \Delta_i = 0)$  is provided in 2.1. Note that in this paper,  $h_3(\mathbf{b}_i)$  could only be  $\mathbf{b}_i$  or  $\mathbf{b}_i\mathbf{b}_i^T$ . And the calculations of  $E[\mathbf{b}_i|\omega_i, \mathbf{y}_i, \Delta_i = 0]$  and  $E[\mathbf{b}_i\mathbf{b}_i^T|\omega_i, \mathbf{y}_i, \Delta_i = 0]$  are provided in 2.1.

## 2.4 Further details for the E-step related to $Q^{(3)}$

We aim to calculate (4), whose proof is provided in 7, and we propose to calculate the nominator and denominator separately. We still note that the denominator is a special case of the nominator when  $h_1$ ,  $h_2$ , and  $h_3$  are all equal to 1. Therefore, we only give the procedure of Monte Carlo integration of the nominator.

$$\begin{aligned} & E[h_1(t_i^*) \cdot h_2(\omega_i) \cdot h_3(\mathbf{b}_i) | t_i^* > t_i, \mathbf{y}_i, \Delta_i = 0] \\ &= \frac{\int_{t_i}^{\infty} \int_0^{e^{t_i^*}} h_1(t_i^*) \cdot h_2(\omega_i) E[h_3(\mathbf{b}_i) | \omega_i, \mathbf{y}_i, \Delta_i = 0] f(\mathbf{y}_i | \omega_i, \Delta_i = 0) f(\omega_i | t_i^*, \Delta_i = 0) f(t_i^* | \Delta_i = 0) d\omega_i dt_i^*}{\int_{t_i}^{\infty} \int_0^{e^{t_i^*}} f(\mathbf{y}_i | \omega_i, \Delta_i = 0) f(\omega_i | t_i^*, \Delta_i = 0) f(t_i^* | \Delta_i = 0) d\omega_i dt_i^*} \end{aligned} \quad (4)$$

In order to calculate  $\int_{t_i}^{\infty} \int_0^{e^{t_i^*}} h_1(t_i^*) \cdot h_2(\omega_i) E[h_3(\mathbf{b}_i) | \omega_i, \mathbf{y}_i, \Delta_i = 0] f(\mathbf{y}_i | \omega_i, \Delta_i = 0) f(\omega_i | t_i^*, \Delta_i = 0) f(t_i^* | \Delta_i = 0) d\omega_i dt_i^*$ , we can use the following procedures. First, for  $j \in \{1, 2, \dots, J\}$ , sample  $t_i^{*(j)} \sim TN(\mu_{tte}, \sigma_{tte}^2, t_i, \infty)$ . Then sample  $\omega_i^{(j)} | t_i^{*(j)} \sim TN(\mu_{\omega}, \sigma_{\omega}^2, 0, e^{t_i^{*(j)}})$ . Finally, we can get  $\int_{t_i}^{\infty} \int_0^{e^{t_i^*}} h_1(t_i^*) \cdot h_2(\omega_i) E[h_3(\mathbf{b}_i) | \omega_i, \mathbf{y}_i, \Delta_i = 0] f(\mathbf{y}_i | \omega_i, \Delta_i = 0) f(\omega_i | t_i^*, \Delta_i = 0) f(t_i^* | \Delta_i = 0) d\omega_i dt_i^* \approx \frac{1}{J} \sum_{j=1}^J h_1(t_i^{*(j)}) \cdot h_2(\omega_i^{(j)}) \cdot E[h_3(\mathbf{b}_i) | \omega_i^{(j)}, \mathbf{y}_i, \Delta_i = 0] \cdot f(\mathbf{y}_i | \omega_i^{(j)}, \Delta_i = 0)$ , where  $f(\mathbf{y}_i | \omega_i^{(j)}, \Delta_i = 0)$  is provided in 2.1. Note that in this paper,  $h_3(\mathbf{b}_i)$  could only be  $\mathbf{b}_i$  or  $\mathbf{b}_i \mathbf{b}_i^T$ . And the calculations of  $E[\mathbf{b}_i | \omega_i, \mathbf{y}_i, \Delta_i = 0]$  and  $E[\mathbf{b}_i \mathbf{b}_i^T | \omega_i, \mathbf{y}_i, \Delta_i = 0]$  are provided in 2.1.

## 2.5 Further details for the E-step related to $Q^{(4)}$

We note that  $\mathbf{b}_{(s),i} \sim N(\boldsymbol{\mu}_{r,(s)}, \boldsymbol{\Sigma}_{r,(s)})$  and  $\mathbf{y}_i | \mathbf{b}_{(s),i} \sim N_{n_i}(\mathbf{X}_{(s),i} \boldsymbol{\beta}_{(s)} + \mathbf{Z}_{(s),i} \mathbf{b}_{(s),i}, \sigma_{y,(s)}^2 \mathbf{I}_{n_i})$ . And using the properties of the multivariate normal distribution, we can get

$$\begin{bmatrix} \mathbf{y}_i \\ \mathbf{b}_{(s),i} - \boldsymbol{\mu}_{r,(s)} \end{bmatrix} \sim N \left( \begin{bmatrix} \mathbf{X}_{(s),i} \boldsymbol{\beta}_{(s)} + \mathbf{Z}_{(s),i} \boldsymbol{\mu}_{r,(s)} \\ 0 \end{bmatrix}, \begin{bmatrix} \sigma_{y,(s)}^2 \mathbf{I}_{n_i} + \mathbf{Z}_{(s),i} \boldsymbol{\Sigma}_{r,(s)} \mathbf{Z}_{(s),i}^T & \mathbf{Z}_{(s),i} \boldsymbol{\Sigma}_{r,(s)} \\ \boldsymbol{\Sigma}_{r,(s)} \mathbf{Z}_{(s),i}^T & \boldsymbol{\Sigma}_{r,(s)} \end{bmatrix} \right).$$

Therefore, based on the properties of the conditional distribution for multivariate normal distribution, we get

$$E[\mathbf{b}_{(s),i} | \mathbf{y}_i, \Delta_i = 1] = \boldsymbol{\mu}_{r,(s)} + \boldsymbol{\Sigma}_{r,(s)} \mathbf{Z}_{(s),i}^T \left( \sigma_{y,(s)}^2 \mathbf{I}_{n_i} + \mathbf{Z}_{(s),i} \boldsymbol{\Sigma}_{r,(s)} \mathbf{Z}_{(s),i}^T \right)^{-1} (\mathbf{y}_i - \mathbf{X}_{(s),i} \boldsymbol{\beta}_{(s)} - \mathbf{Z}_{(s),i} \boldsymbol{\mu}_{r,(s)}),$$

and

$$\text{Var}(\mathbf{b}_{(s),i} - \boldsymbol{\mu}_{r,(s)} | \Delta_1 = 1, \mathbf{y}_i) = \boldsymbol{\Sigma}_{r,(s)} - \boldsymbol{\Sigma}_{r,(s)} \mathbf{Z}_{(s),i}^T \left( \sigma_{y,(s)}^2 \mathbf{I}_{n_i} + \mathbf{Z}_{(s),i} \boldsymbol{\Sigma}_{r,(s)} \mathbf{Z}_{(s),i}^T \right)^{-1} \mathbf{Z}_{(s),i} \boldsymbol{\Sigma}_{r,(s)}.$$

We note that  $E_1[\mathbf{b}_{(s),i}] = E[\mathbf{b}_{(s),i} | \mathbf{y}_i, \Delta_i = 1]$  and  $E_1[(\mathbf{b}_{(s),i} - \boldsymbol{\mu}_{r,(s)})^{\otimes 2}] = \text{Var}(\mathbf{b}_{(s),i} - \boldsymbol{\mu}_{r,(s)} | \Delta_1 = 1, \mathbf{y}_i) + (E_1[\mathbf{b}_{(s),i} - \boldsymbol{\mu}_{r,(s)}])^{\otimes 2}$ , which give us the closed form of the expectations.

### 3 Details for the M-steps

#### 3.1 Closed-form solutions for some parameters in the M-step

We focus on the parameters that have closed-form solutions in the M-step. The only parameter involved in  $Q^{(1)}$  is  $\pi_{(s)}$ . To obtain the MLE, let  $\frac{\partial Q}{\partial \pi_{(s)}} = 0$ , we get

$$\hat{\pi}_{(s)} = n^{-1} \sum_{i=1}^n E^{(>)}[\Delta_i](1 - \nu_i).$$

The parameter  $\hat{\pi}_{(s)}$  represents the mean probability that a given subject is both censored and belongs to the stable group.

The parameters involved in  $Q^{(2)}$  and  $Q^{(3)}$  consist of six components, all of which belong to the change-point group. These include the parameters for the time-to-event model ( $\gamma$  and  $\sigma_{tte}$ ), the parameters for the random effects model ( $\mu_r$  and  $\Sigma_r$ ), and the parameters for the longitudinal model ( $\beta$  and  $\sigma_y$ ). Of these parameters,  $\gamma$ ,  $\sigma_{tte}$ ,  $\beta$ , and  $\sigma_y$  have closed-form solutions in the M-step. The scalar forms of these expressions, which provide greater clarity on how the E-step results are utilized in the M-step, are detailed in 3.2.

Maximizing the Q function with respect to  $\gamma$  in the time-to-event model gives

$$\hat{\gamma} = \left( \mathbf{W}^T \left( \mathbf{V} + E^{(>)}[\mathbf{V}^{(c)}] \right) \mathbf{W} \right)^{-1} \mathbf{W}^T \left( \mathbf{V} \mathbf{t} + E^{(>)}[\mathbf{V}^{(c)} \mathbf{t}^*] \right),$$

where  $\mathbf{W} = [\mathbf{w}_1, \mathbf{w}_2, \dots, \mathbf{w}_n]^T$  represents the  $n \times p_{tte}$  matrix of covariates,  $\mathbf{t} = [t_1, t_2, \dots, t_n]^T$ ,  $\mathbf{t}^* = [t_1^*, t_2^*, \dots, t_n^*]^T$ ,  $\mathbf{V} = \text{diag}\{\nu_i, i = 1, \dots, n\}$ , and  $\mathbf{V}^{(c)} = \text{diag}\{(1 - \nu_i)(1 - \Delta_i), i = 1, \dots, n\}$ . The estimator  $\hat{\gamma}$  integrates observed data with a weight of  $\nu_i$  and incorporates expected contributions from the censored change-point group with a weight of  $(1 - \nu_i)E^{(>)}[1 - \Delta_i]$ .

The maximizer for  $\sigma_{tte}^2$  is given by

$$\hat{\sigma}_{tte}^2 = \frac{(\mathbf{t} - \mathbf{W}\gamma)^T \mathbf{V} (\mathbf{t} - \mathbf{W}\gamma) + E^{(>)}[(\mathbf{t}^* - \mathbf{W}\gamma)^T \mathbf{V}^{(c)} (\mathbf{t}^* - \mathbf{W}\gamma)]}{\text{tr}(\mathbf{V} + E^{(>)}[\mathbf{V}^{(c)}])}.$$

This formulation enables a combined estimation of variance in both observed data and expected contributions from censored subjects who is in the change-point group.

In terms of the parameter  $\beta$  in the longitudinal outcome for subjects in the change-point group, we have

$$\hat{\beta} = \left( \mathbf{X}^T \left( \mathbf{V}_b + E^{(>)}[\mathbf{V}_b^{(c)}] \right) \mathbf{X} \right)^{-1} \mathbf{X}^T \left( \mathbf{V}_b \left( \mathbf{y} - E_0^{(=)}[\mu \mathbf{z} \mathbf{b}] \right) + E^{(>)}[\mathbf{V}_b^{(c)}] \left( \mathbf{y} - E_0^{(>)}[\mu \mathbf{z} \mathbf{b}] \right) \right),$$

where  $\mathbf{X} = [\mathbf{X}_1^T, \mathbf{X}_2^T, \dots, \mathbf{X}_n^T]^T$  is the  $N \times p_{long}$  design matrix for fixed effects,  $\mathbf{y} = [\mathbf{y}_1^T, \mathbf{y}_2^T, \dots, \mathbf{y}_n^T]^T$  is the  $N$ -dimensional vector of observed longitudinal outcomes,  $\mathbf{V}_b = \text{blkdiag}\{\nu_i \mathbf{I}_{n_i}, i = 1, \dots, n\}$ ,  $\mathbf{V}_b^{(c)} = \text{blkdiag}\{(1 - \nu_i)(1 - \Delta_i) \mathbf{I}_{n_i}, i = 1, \dots, n\}$ , and  $\mu \mathbf{z} \mathbf{b} = [(\mathbf{Z}_1 \mathbf{b}_1)^T, (\mathbf{Z}_2 \mathbf{b}_2)^T, \dots, (\mathbf{Z}_n \mathbf{b}_n)^T]^T$ . The estimator  $\hat{\beta}$  incorporates both observed and expected contributions from censored subjects, and is a sort of weighted average between the contributions from these two groups.

An estimator of the variance  $\sigma_y^2$  of the longitudinal outcome for the subjects in the change-point group may be obtained as

$$\hat{\sigma}_y^2 = \frac{E_0^{(=)} [(\mathbf{y} - \boldsymbol{\mu}_{\mathbf{Z}\mathbf{b}} - \mathbf{X}\boldsymbol{\beta})^T \mathbf{V}_b (\mathbf{y} - \boldsymbol{\mu}_{\mathbf{Z}\mathbf{b}} - \mathbf{X}\boldsymbol{\beta})] + E^{(>)} [(\mathbf{y} - \boldsymbol{\mu}_{\mathbf{Z}\mathbf{b}} - \mathbf{X}\boldsymbol{\beta})^T \mathbf{V}_b^{(c)} (\mathbf{y} - \boldsymbol{\mu}_{\mathbf{Z}\mathbf{b}} - \mathbf{X}\boldsymbol{\beta})]}{\text{tr}(\mathbf{V}_b + E^{(>)} [\mathbf{V}_b^{(c)}])}.$$

This expression provides a weighted estimator for  $\hat{\sigma}_y^2$ , wherein the variance combines observed outcomes with expected outcomes from censored cases.

There are 4 parameters involved in  $Q^{(4)}$ , which correspond to the individuals in the stable group. We list the matrix form here and still provide the scalar form in 3.2. First, we set  $\frac{\partial Q}{\partial \boldsymbol{\mu}_{r,(s)}}$  and  $\frac{\partial Q}{\partial \boldsymbol{\Sigma}_{r,(s)}^{-1}}$  equal to 0, to obtain (5) and (6).

$$\hat{\boldsymbol{\mu}}_{r,(s)} = [\mathbf{J}_n^T E^{(>)} [\mathbf{V}^{(s)}] \mathbf{J}_n]^{-1} E^{(>)} [\mathbf{b}_{(s)}^T \mathbf{V}^{(s)} \mathbf{J}_n], \quad (5)$$

where  $\mathbf{J}_n$  is a  $n$  dimensional vector of 1,  $\mathbf{V}^{(s)} = \text{diag}\{(1 - \nu_i)\Delta_i, i = 1, \dots, n\}$ , and  $\mathbf{b}_{(s)} = (\mathbf{b}_{(s),1}, \mathbf{b}_{(s),2}, \dots, \mathbf{b}_{(s),n})^T$ .

$$\hat{\boldsymbol{\Sigma}}_{r,(s)} = \frac{(\mathbf{b}_{(s)} - \boldsymbol{\mu}_{\mathbf{b}_{(s)}})^T E^{(>)} [\mathbf{V}^{(s)}] (\mathbf{b}_{(s)} - \boldsymbol{\mu}_{\mathbf{b}_{(s)}})}{\text{tr}(E^{(>)} [\mathbf{V}^{(s)}])}, \quad (6)$$

where  $\boldsymbol{\mu}_{\mathbf{b}_{(s)}}$  is formed by column-stacking  $\boldsymbol{\mu}_{r,(s)}^T$  repeated  $n$  times. From (5) and (6), it is evident that the M-step for the random effect in the stable group extends the basic random effect model by incorporating the weight  $(1 - \nu_i)E^{(>)}[\Delta_i]$ , which adjusts for the probability that each subject belongs to the stable group. Additionally, we set  $\frac{\partial Q}{\partial \boldsymbol{\beta}_{(s)}}$  and  $\frac{\partial Q}{\partial \sigma_{y,(s)}^2}$  to be 0, and obtain (7) and (8).

$$\hat{\boldsymbol{\beta}}_{(s)} = \left( \mathbf{X}_{(s)}^T E^{(>)} [\mathbf{V}_b^{(s)}] \mathbf{X}_{(s)} \right)^{-1} \mathbf{X}_{(s)}^T E^{(>)} [\mathbf{V}_b^{(s)}] \left( \mathbf{y} - E_1^{(>)} [\boldsymbol{\mu}_{\mathbf{Z}_{(s)}} \mathbf{b}_{(s)}] \right), \quad (7)$$

where  $\mathbf{X}_{(s)} = [\mathbf{X}_{(s),1}^T, \mathbf{X}_{(s),2}^T, \dots, \mathbf{X}_{(s),n}^T]^T$  is the  $(\sum_{i=1}^n n_i) \times p_{(s)}$  design matrix for the stable group,  $\mathbf{V}_b^{(s)} = \text{blkdiag}\{(1 - \nu_i)\Delta_i \mathbf{I}_{n_i}, i = 1, \dots, n\}$ ,  $\mathbf{y} = [\mathbf{y}_1^T, \mathbf{y}_2^T, \dots, \mathbf{y}_n^T]^T$  is still the  $N$ -dimensional vector of observed longitudinal outcomes,  $\boldsymbol{\mu}_{\mathbf{Z}_{(s)}} \mathbf{b}_{(s)} = [(\mathbf{Z}_{(s),1} \mathbf{b}_{(s),1})^T, (\mathbf{Z}_{(s),2} \mathbf{b}_{(s),2})^T, \dots, (\mathbf{Z}_{(s),n} \mathbf{b}_{(s),n})^T]^T$  is the vector of random effect contributions for the subjects in the stable group.

$$\hat{\sigma}_{y,(s)}^2 = \frac{E^{(>)} [(\mathbf{y} - \mathbf{X}_{(s)}\boldsymbol{\beta}_{(s)} - \boldsymbol{\mu}_{\mathbf{Z}_{(s)}} \mathbf{b}_{(s)})^T \mathbf{V}_b^{(s)} (\mathbf{y} - \mathbf{X}_{(s)}\boldsymbol{\beta}_{(s)} - \boldsymbol{\mu}_{\mathbf{Z}_{(s)}} \mathbf{b}_{(s)})]}{\text{tr}(E^{(>)} [\mathbf{V}^{(s)}])}. \quad (8)$$

Similarly, (7) and (8) indicate that the parameters in the longitudinal component for the stable group extend the basic random effects model, with adjustments that weight each subject's contribution by  $(1 - \nu_i)E^{(>)}[\Delta_i]$ .

### 3.2 Closed-form solutions for some parameters in the M-step in scalar form

To clarify how the quantities derived in the E-step are applied in the M-step, we present the scalar forms of the M-step updates for parameters with closed-form solutions.

$$\hat{\gamma} = \left( \sum_{i=1}^n \left( \nu_i \mathbf{w}_i \mathbf{w}_i^T + (1 - \nu_i) E^{(>)} [1 - \Delta_i] \mathbf{w}_i \mathbf{w}_i^T \right) \right)^{-1} \left( \sum_{i=1}^n \left( \nu_i \mathbf{w}_i t_i + (1 - \nu_i) E^{(>)} [1 - \Delta_i] \mathbf{w}_i E_0^{(>)} [t_i^*] \right) \right),$$

$$\hat{\sigma}_{tte}^2 = \frac{\sum_{i=1}^n \left( \nu_i (t_i - \mathbf{w}_i^T \boldsymbol{\gamma})^2 + (1 - \nu_i) E^{(>)} [1 - \Delta_i] E_0^{(>)} [(t_i - \mathbf{w}_i^T \boldsymbol{\gamma})^2] \right)}{\sum_{i=1}^n \left( \nu_i + (1 - \nu_i) E^{(>)} [1 - \Delta_i] \right)},$$

$$\begin{aligned} \hat{\boldsymbol{\beta}} = & \left( \sum_{i=1}^n \left( \nu_i \mathbf{X}_i^T \mathbf{X}_i + (1 - \nu_i) E^{(>)} [1 - \Delta_i] \mathbf{X}_i^T \mathbf{X}_i \right) \right)^{-1} \\ & \times \left( \sum_{i=1}^n \left( \nu_i \mathbf{X}_i^T (\mathbf{y}_i - E_0^{(=)} [\mathbf{Z}_i \mathbf{b}_i]) + (1 - \nu_i) E^{(>)} [1 - \Delta_i] \mathbf{X}_i^T (\mathbf{y}_i - E_0^{(>)} [\mathbf{Z}_i \mathbf{b}_i]) \right) \right), \end{aligned}$$

$$\hat{\sigma}_y^2 = \frac{\sum_{i=1}^n \nu_i E_0^{(=)} [\|\mathbf{y}_i - \mathbf{Z}_i \mathbf{b}_i - \mathbf{X}_i \boldsymbol{\beta}\|_2^2] + \sum_{i=1}^n (1 - \nu_i) E^{(>)} [1 - \Delta_i] E_0^{(>)} [\|\mathbf{y}_i - \mathbf{Z}_i \mathbf{b}_i - \mathbf{X}_i \boldsymbol{\beta}\|_2^2]}{\sum_{i=1}^n \left( \nu_i + (1 - \nu_i) E^{(>)} [1 - \Delta_i] \right) n_i},$$

$$\hat{\boldsymbol{\mu}}_{r,(s)} = \left[ \sum_{i=1}^n (1 - \nu_i) E^{(>)} [\Delta_i] \right]^{-1} \left[ \sum_{i=1}^n (1 - \nu_i) E^{(>)} [\Delta_i] E_1 [\mathbf{b}_{(s),i}] \right],$$

$$\hat{\boldsymbol{\Sigma}}_{r,(s)} = \frac{\sum_{i=1}^n (1 - \nu_i) E^{(>)} [\Delta_i] E_1 [(\mathbf{b}_{(s),i} - \boldsymbol{\mu}_{r,(s)})^{\otimes 2}]}{\sum_{i=1}^n (1 - \nu_i) E^{(>)} [\Delta_i]},$$

$$\hat{\boldsymbol{\beta}}_{(s)} = \left( \sum_{i=1}^n (1 - \nu_i) E^{(>)} [\Delta_i] \mathbf{X}_{(s),i} \mathbf{X}_{(s),i}^T \right)^{-1} \left( \sum_{i=1}^n (1 - \nu_i) E^{(>)} [\Delta_i] \mathbf{X}_{(s),i}^T (\mathbf{y}_i - \mathbf{Z}_{(s),i} E_1 [\mathbf{b}_{(s),i}]) \right),$$

$$\hat{\sigma}_{y,(s)}^2 = \frac{\sum_{i=1}^N (1 - \nu_i) E^{(>)} [\Delta_i] \text{tr} \{ E_1 [(\mathbf{y}_i - \mathbf{X}_{(s),i} \boldsymbol{\beta}_{(s)} - \mathbf{Z}_{(s),i} \mathbf{b}_{(s),i})^{\otimes 2}] \}}{\sum_{i=1}^N (1 - \nu_i) E^{(>)} [\Delta_i] n_i}.$$

### 3.3 The derivative of Q function with respect to $\boldsymbol{\mu}_r$ and $\boldsymbol{\Sigma}_r$

#### 3.3.1 Calculation of $\frac{\partial Q}{\partial \boldsymbol{\mu}_r}$

We first notice that  $\frac{\partial \mu_\omega}{\partial \boldsymbol{\mu}_r} = (1, 0, 0, 0)^T$ . And we denote  $g_1(t_i^*) = \frac{\phi(\frac{e^{t_i^*} - \mu_\omega}{\sigma_\omega}) - \phi(\frac{-\mu_\omega}{\sigma_\omega})}{\left( \Phi(\frac{e^{t_i^*} - \mu_\omega}{\sigma_\omega}) - \Phi(\frac{-\mu_\omega}{\sigma_\omega}) \right) \sigma_\omega}$ . Then we get

$$\begin{aligned} \frac{\partial Q}{\partial \boldsymbol{\mu}_r} = & \sum_{i=1}^n \nu_i \left( \boldsymbol{\Sigma}_r^{-1} \left[ E_0^{(=)} [\mathbf{r}_i] - \boldsymbol{\mu}_r \right] + g_1(t_i) \cdot \frac{\partial \mu_\omega}{\partial \boldsymbol{\mu}_r} \right) \\ & + \sum_{i=1}^n (1 - \nu_i) \left( \boldsymbol{\Sigma}_r^{-1} \left[ E_0^{(>)} [\mathbf{r}_i] - \boldsymbol{\mu}_r \right] + E_0^{(>)} [g_1(t_i^*)] \cdot \frac{\partial \mu_\omega}{\partial \boldsymbol{\mu}_r} \right). \end{aligned}$$

### 3.3.2 Calculation of $\frac{\partial Q}{\partial \text{vech}(\mathbf{P}_r)}$

**Reparametrization of  $\Sigma_r$**  To deal with positive definite matrix  $\Sigma_r$ , we first parameterize  $\mathbf{P}_r = \begin{pmatrix} p_{11} & 0 & 0 & 0 \\ p_{21} & p_{22} & 0 & 0 \\ p_{31} & p_{32} & p_{33} & 0 \\ p_{41} & p_{42} & p_{43} & p_{44} \end{pmatrix}$ .

Then we let  $\mathbf{O}_r = \begin{pmatrix} e^{p_{11}} & 0 & 0 & 0 \\ p_{21} & e^{p_{22}} & 0 & 0 \\ p_{31} & p_{32} & e^{p_{33}} & 0 \\ p_{41} & p_{42} & p_{43} & e^{p_{44}} \end{pmatrix} \stackrel{\text{denote}}{=} \begin{pmatrix} o_{11} & 0 & 0 & 0 \\ o_{21} & o_{22} & 0 & 0 \\ o_{31} & o_{32} & o_{33} & 0 \\ o_{41} & o_{42} & o_{43} & o_{44} \end{pmatrix}$ , and let  $\Sigma_r = \mathbf{O}_r \mathbf{O}_r^T$ . In order to optimize  $\Sigma_r$ , we just need to optimize  $\text{vech}(\mathbf{P}_r)$ .

**Detailed calculations based on chain rule** We denote  $B_i^{(2)} = -\frac{1}{2} \log(|\Sigma_r|) - \frac{1}{2} E_0^{(-)}[(\mathbf{r}_i - \boldsymbol{\mu}_r)^T \Sigma_r^{-1} (\mathbf{r}_i - \boldsymbol{\mu}_r)]$ . We first want to find  $\frac{\partial B_i^{(2)}}{\partial \text{vech}(\mathbf{P}_r)}$ .

We first derive (9) based on the chain rule.

$$\frac{\partial B_i^{(2)}}{\partial \text{vech}(\mathbf{P}_r)} = \frac{\partial \text{vech}(\mathbf{O}_r)^T}{\partial \text{vech}(\mathbf{P}_r)} \frac{\partial B_i^{(2)}}{\partial \text{vech}(\mathbf{O}_r)} = \frac{\partial \text{vech}(\mathbf{O}_r)^T}{\partial \text{vech}(\mathbf{P}_r)} \frac{\partial \text{vech}(\Sigma_r)^T}{\partial \text{vech}(\mathbf{O}_r)} \frac{\partial B_i^{(2)}}{\partial \text{vech}(\Sigma_r)}. \quad (9)$$

Obviously, based on the relationship between  $\mathbf{O}_r$  and  $\mathbf{P}_r$  we have

$$\frac{\partial \text{vech}(\mathbf{O}_r)^T}{\partial \text{vech}(\mathbf{P}_r)} = \text{diag}(o_{11}, 1, 1, 1, o_{22}, 1, 1, o_{33}, 1, o_{44}). \quad (10)$$

And we can get (11) based on Proposition 1 in Section 7, where  $\mathbf{L}$ ,  $\mathbf{K}$ ,  $\mathbf{T}$ , and  $\mathbf{D}$  are defined in Proposition 1.

$$\frac{\partial \text{vech}(\Sigma_r)^T}{\partial \text{vech}(\mathbf{O}_r)} = [\mathbf{L}_4 (\mathbf{O}_r \otimes \mathbf{I} + \mathbf{I} \otimes \mathbf{O}_r \cdot \mathbf{K}_4) \mathbf{T}_4 \mathbf{D}_4]^T. \quad (11)$$

To calculate  $\frac{\partial B_i^{(2)}}{\partial \text{vech}(\Sigma_r)}$ , we first calculate  $\frac{\partial B_i^{(2)}}{\partial \Sigma_r}$  as

$$\frac{\partial B_i^{(2)}}{\partial \Sigma_r} = -\frac{1}{2} \left( \Sigma_r^{-1} - \Sigma_r^{-1} E_0^{(-)}[(\mathbf{r}_i - \boldsymbol{\mu}_r)(\mathbf{r}_i - \boldsymbol{\mu}_r)^T] \Sigma_r^{-1} \right).$$

Since  $\Sigma_r$  is symmetric, we can get

$$\frac{\partial B_i^{(2)}}{\partial \text{vech}(\Sigma_r)} = \text{vech} \left( \frac{\partial B_i^{(2)}}{\partial \Sigma_r} + \left( \frac{\partial B_i^{(2)}}{\partial \Sigma_r} \right)^T - \text{diag} \left( \frac{\partial B_i^{(2)}}{\partial \Sigma_r} \right) \right). \quad (12)$$

Therefore, we get the results of (9) based on (10), (11), and (12).

Similarly, for censored subjects, we denote  $B_i^{(3)} = -\frac{1}{2} \log(|\Sigma_r|) - \frac{1}{2} E_0^{(>)}[(\mathbf{r}_i - \boldsymbol{\mu}_r)^T \Sigma_r^{-1} (\mathbf{r}_i - \boldsymbol{\mu}_r)]$ , and get

$$\frac{\partial B_i^{(3)}}{\partial \text{vech}(\mathbf{P}_r)} = \frac{\partial \text{vech}(\mathbf{O}_r)^T}{\partial \text{vech}(\mathbf{P}_r)} \frac{\partial B_i^{(3)}}{\partial \text{vech}(\mathbf{O}_r)} = \frac{\partial \text{vech}(\mathbf{O}_r)^T}{\partial \text{vech}(\mathbf{P}_r)} \frac{\partial \text{vech}(\mathbf{\Sigma}_r)^T}{\partial \text{vech}(\mathbf{O}_r)} \frac{\partial B_i^{(3)}}{\partial \text{vech}(\mathbf{\Sigma}_r)}.$$

We denote  $C_i^{(2)} = -\log \left( \Phi\left(\frac{e^{t_i} - \mu_\omega}{\sigma_\omega}\right) - \Phi\left(\frac{-\mu_\omega}{\sigma_\omega}\right) \right)$  and  $C_i^{(3)} = -E_0^{(>)} \left[ \log \left( \Phi\left(\frac{e^{t_i} - \mu_\omega}{\sigma_\omega}\right) - \Phi\left(\frac{-\mu_\omega}{\sigma_\omega}\right) \right) \right]$ , which also involve the element of  $\mathbf{P}_r$ . We notice that  $\sigma_\omega^2 = o_{11}^2 = e^{2p_{11}}$ . Therefore,  $\frac{\partial \sigma_\omega}{\partial \text{vech}(\mathbf{P}_r)} = (\sigma_\omega, 0, 0, 0, 0, 0, 0, 0, 0)^T$ .

We also denote  $g_2(t_i^*) = \frac{\phi\left(\frac{e^{t_i^*} - \mu_\omega}{\sigma_\omega}\right) - \phi\left(\frac{-\mu_\omega}{\sigma_\omega}\right)}{\Phi\left(\frac{e^{t_i^*} - \mu_\omega}{\sigma_\omega}\right) - \Phi\left(\frac{-\mu_\omega}{\sigma_\omega}\right)}$ . Therefore, we have (13) and (14).

$$\frac{\partial C_i^{(2)}}{\partial \text{vech}(\mathbf{P}_r)} = -g_2(t_i) \cdot \frac{\partial \sigma_\omega}{\partial \text{vech}(\mathbf{P}_r)}, \quad (13)$$

$$\frac{\partial C_i^{(3)}}{\partial \text{vech}(\mathbf{P}_r)} = -E_0^{(>)} [g_2(t_i^*)] \cdot \frac{\partial \sigma_\omega}{\partial \text{vech}(\mathbf{P}_r)}. \quad (14)$$

Our final goal  $\frac{\partial Q}{\partial \text{vech}(\mathbf{P}_r)}$  can be calculated as follows.

$$\frac{\partial Q}{\partial \text{vech}(\mathbf{P}_r)} = \sum_{i=1}^n \nu_i \left( \frac{\partial B_i^{(2)}}{\partial \text{vech}(\mathbf{P}_r)} + \frac{\partial C_i^{(2)}}{\partial \text{vech}(\mathbf{P}_r)} \right) + \sum_{i=1}^n (1 - \nu_i) \left( \frac{\partial B_i^{(3)}}{\partial \text{vech}(\mathbf{P}_r)} + \frac{\partial C_i^{(3)}}{\partial \text{vech}(\mathbf{P}_r)} \right).$$

## 4 Details for the longitudinal trajectory estimations

### 4.1 The derivation for the longitudinal trajectory estimations

$$\begin{aligned} E[y|s, \boldsymbol{\theta}] &= E[E[y|\mathbf{X}, \mathbf{X}_{(s)}, s, \Delta, \boldsymbol{\theta}]|s, \boldsymbol{\theta}] \\ &= \pi_{(s)} E[y|\mathbf{X}_{(s)}, s, \Delta = 1, \boldsymbol{\theta}] + (1 - \pi_{(s)}) E[y|\mathbf{X}, s, \Delta = 0, \boldsymbol{\theta}] \\ &= \pi_{(s)} (E[\mathbf{X}_{(s)}] \boldsymbol{\beta}_{(s)} + E[\mathbf{Z}_{(s)} \mathbf{b}_{(s)}|s, \boldsymbol{\theta}]) + (1 - \pi_{(s)}) (E[\mathbf{X}] \boldsymbol{\beta} + E[\mathbf{Z} \mathbf{b}|s, \boldsymbol{\theta}]) \\ &= \pi_{(s)} (E[\mathbf{X}_{(s)}] \boldsymbol{\beta}_{(s)} + \mu_{b_{(s)},0} + \mu_{b_{(s)},1} s) \\ &\quad + (1 - \pi_{(s)}) (E[\mathbf{X}] \boldsymbol{\beta} + E[b_0 + b_1(s - \omega)I(s \leq \omega) + b_2(s - \omega)I(s > \omega)|\boldsymbol{\theta}]) \\ &\approx \pi_{(s)} (\bar{\mathbf{X}}_{(s)} \boldsymbol{\beta}_{(s)} + \mu_{b_{(s)},0} + \mu_{b_{(s)},1} s) \\ &\quad + (1 - \pi_{(s)}) (\bar{\mathbf{X}} \boldsymbol{\beta} + E[b_0 + b_1(s - \omega)I(s \leq \omega) + b_2(s - \omega)I(s > \omega)|\boldsymbol{\theta}]). \end{aligned}$$

The Monte Carlo sampling procedures to estimate  $E[b_0 + b_1(s - \omega)I(s \leq \omega) + b_2(s - \omega)I(s > \omega)|\boldsymbol{\theta}]$  are further provided in Section 4.2.

### 4.2 Monte Carlo sampling for the longitudinal trajectory estimations

We provide the Monte Carlo sampling procedures for calculating  $E[b_0 + b_1(s - \omega)I(s \leq \omega) + b_2(s - \omega)I(s > \omega)|\boldsymbol{\theta}]$  in this section. We first note that the marginal distributions of  $\mathbf{r}$  (i.e.,  $\omega$  and  $\mathbf{b}$ ) are not trivial since we only

know conditional on the progression time  $t$ ,  $\omega|t$  follows a truncated normal distribution. Therefore, we adapt the Monte Carlo approach to estimate the expectation. Specifically, for  $j \in \{1, 2, \dots, J\}$ , where  $J$  is the predefined sampling repetition number, we sample  $t^{(j)} \sim N(E[\mathbf{w}]^T \boldsymbol{\gamma}, \sigma_{tte}^2)$ , and then we sample  $(\omega^{(j)}, b_0^{(j)}, b_1^{(j)}, b_2^{(j)})^T | t^{(j)} \sim PTMVN(\boldsymbol{\mu}_r, \boldsymbol{\Sigma}_r, 0, e^{t^{(j)}})$ . Note that similarly to  $E[\mathbf{X}]$ , we still substitute  $E[\mathbf{w}]$  with  $\bar{\mathbf{w}}$  since  $\mathbf{w}$  also only consists of the measurements at baseline in our application. Using the sampled  $\mathbf{r}^{(j)}$ , or more specifically  $(\omega^{(j)}, b_0^{(j)}, b_1^{(j)}, b_2^{(j)})$ , we can estimate the quantity  $E[y|s, \boldsymbol{\theta}]$  by plugging them into the expression and averaging over the realizations.

## 5 Details in simulation

### 5.1 The parameters used in the simulation

Table 1 summarizes the parameters utilized in our simulation studies. The values enclosed in curly braces indicate different scenarios considered in the analysis.

| $\pi_{(s)}$       | $\beta_1$ | $\sigma_{tte}$ | $\beta_y$ | $\sigma_y$ | $\boldsymbol{\mu}_r$                                                                                                                | $\boldsymbol{\Sigma}_r$                                                                                                                                                | $\beta_{(s),1}$ | $\sigma_{y,(s)}$ | $\boldsymbol{\mu}_{r,(s)}$                   | $\boldsymbol{\Sigma}_{r,(s)}$                                    |
|-------------------|-----------|----------------|-----------|------------|-------------------------------------------------------------------------------------------------------------------------------------|------------------------------------------------------------------------------------------------------------------------------------------------------------------------|-----------------|------------------|----------------------------------------------|------------------------------------------------------------------|
| $\{0, 0.2, 0.4\}$ | -0.1      | 1.0            | -0.1      | 0.1        | $\left\{ \begin{bmatrix} 0.3 \\ 0.0 \\ -0.3 \\ 0.3 \end{bmatrix}, \begin{bmatrix} 0.5 \\ 0.0 \\ -0.5 \\ 0.5 \end{bmatrix} \right\}$ | $\begin{bmatrix} 0.041 & -0.040 & -0.021 & -0.061 \\ -0.040 & 0.074 & 0.038 & 0.078 \\ -0.021 & 0.038 & 0.053 & 0.058 \\ -0.061 & 0.078 & 0.058 & 0.171 \end{bmatrix}$ | -0.1            | 0.1              | $\begin{bmatrix} -0.5 \\ -0.1 \end{bmatrix}$ | $\begin{bmatrix} 0.041 & -0.021 \\ -0.021 & 0.037 \end{bmatrix}$ |

Table 1: Parameters used for the simulation study.

### 5.2 Other simulation results

Figures 1 and 2 represent the simulation results when  $n = 100$  and  $n = 500$ , separately. These results closely resemble those for  $n = 200$ , as shown in the main text.

## 6 The overall estimations of the parameters in the EMPOWER study

### 6.1 Overall change point, pre- and post-slope calculation

To provide an intuitive summary of the estimated marginal longitudinal trajectory ( $E[y|s, \boldsymbol{\theta}]$ ), we propose a method to estimate an overall change point ( $\omega^{(OE)}$ ), an overall pre-slope ( $b_1^{(OE)}$ ), and an overall post-slope ( $b_2^{(OE)}$ ). We omit  $\boldsymbol{\theta}$  in this section for brevity.

First, the overall estimation of the change point,  $\omega^{(OE)}$ , is identified as follows. If  $E[y|s]$  exhibits a consistent decline or is monotonically non-increasing across the interest time frame,  $\omega^{(OE)}$  is set to the last time point

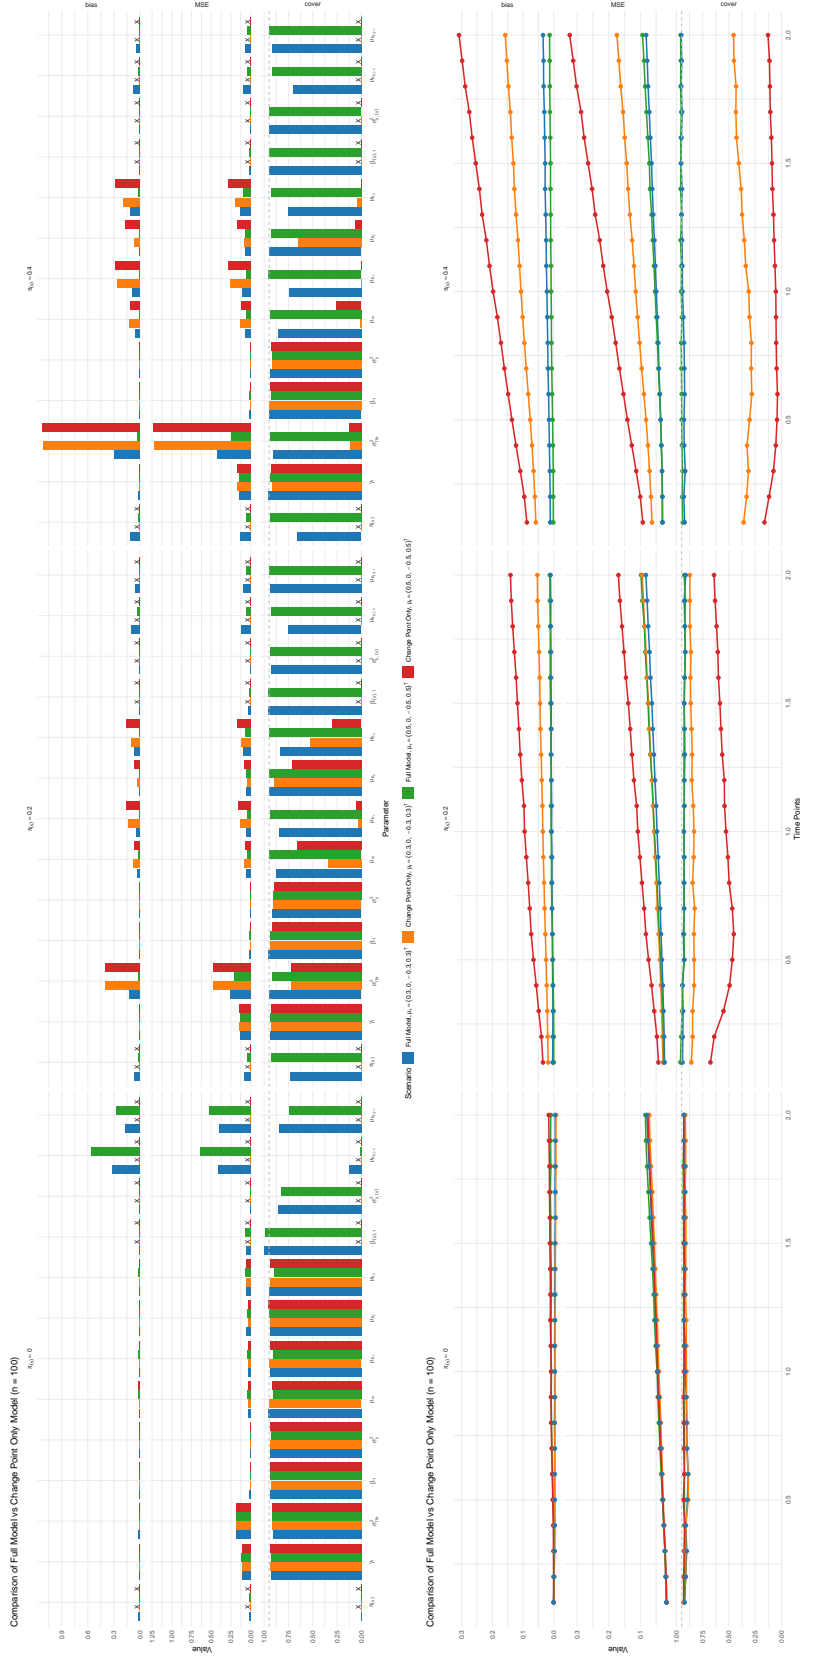

Figure 1: Evaluations for Parameter Estimations and Longitudinal Trajectory Estimations Under Different Scenarios ( $n = 100$ ). The “X” marks indicate the absence of specific parameters in certain models.

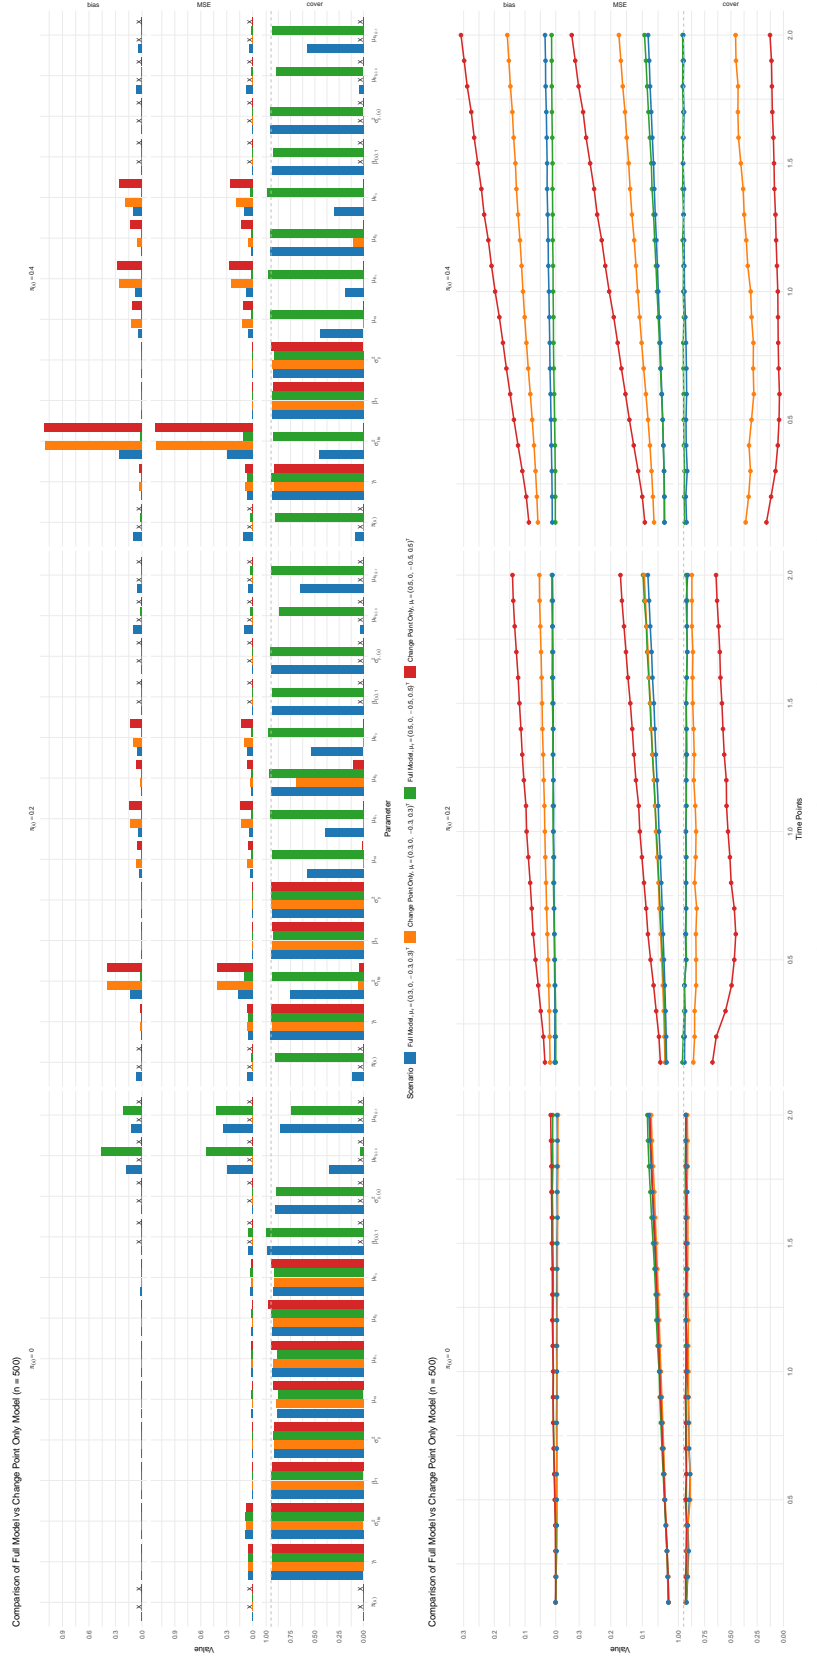

Figure 2: Evaluations for Parameter Estimations and Longitudinal Trajectory Estimations Under Different Scenarios ( $n = 500$ ). The “X” marks indicate the absence of specific parameters in certain models.

of this frame. Otherwise,  $\omega^{(\text{OE})}$  is identified as the earliest time point  $s$  at which  $E[y|s]$  exhibits an increase following any initial non-increasing period.

Subsequently, the overall pre-slope ( $b_1^{(\text{OE})}$  for  $s \leq \omega^{(\text{OE})}$ ) and overall post-slope ( $b_2^{(\text{OE})}$  for  $s > \omega^{(\text{OE})}$ ) are estimated. If  $\omega^{(\text{OE})}$  is set to the last time point of the interest time frame,  $b_2^{(\text{OE})}$  is assigned a value of zero, and  $b_1^{(\text{OE})}$  is estimated from the segment  $s \leq \omega^{(\text{OE})}$  (e.g., via linear regression of  $E[y|s] - E[y|\omega^{(\text{OE})}]$  on  $(s - \omega^{(\text{OE})})I(s \leq \omega^{(\text{OE})})$  without an intercept). In other cases where  $\omega^{(\text{OE})}$  is not the terminal point, both slopes are estimated by fitting a continuous piecewise linear regression model specified as

$$E[y|s] - E[y|\omega^{(\text{OE})}] = b_1^{(\text{OE})}(s - \omega^{(\text{OE})})I(s \leq \omega^{(\text{OE})}) + b_2^{(\text{OE})}(s - \omega^{(\text{OE})})I(s > \omega^{(\text{OE})}) + \epsilon^{(\text{OE})},$$

where  $\epsilon^{(\text{OE})}$  follows a normal distribution. This formulation ensures continuity of the two linear segments at the change point. Confidence intervals for these derived parameters are obtained using the bootstrap method.

## 6.2 The overall estimations in the EMPOWER study

Table 2 gives the parameter estimates by applying our proposed model to the EMPOWER study.

|                      |              | Full                    | Subgroup                           |                              |                          |
|----------------------|--------------|-------------------------|------------------------------------|------------------------------|--------------------------|
|                      |              |                         | $50\% \leq \text{PD-L1} \leq 60\%$ | $60\% < \text{PD-L1} < 90\%$ | $\text{PD-L1} \geq 90\%$ |
| Overall change point | Cemiplimab   | 0.556 (0.394, 0.674)    | 0.37 (0.162, 0.611)                | 0.611 (0.441, 1.37)          | 0.896 (0.578, 1.37)      |
|                      | Chemotherapy | 0.301 (0.247, 0.359)    | 0.247 (0.173, 0.321)               | 0.422 (0.266, 0.638)         | 0.249 (0.173, 0.359)     |
| Overall pre-slope    | Cemiplimab   | -0.174 (-0.217, -0.142) | -0.101 (-0.17, -0.066)             | -0.2 (-0.244, -0.088)        | -0.155 (-0.264, -0.071)  |
|                      | Chemotherapy | -0.149 (-0.185, -0.116) | -0.135 (-0.192, -0.1)              | -0.174 (-0.244, -0.129)      | -0.125 (-0.198, -0.076)  |
| Overall post-slope   | Cemiplimab   | 0.091 (0.041, 0.206)    | 0.204 (0.099, 0.379)               | 0.064 (0, 0.213)             | 0.003 (0, 0.073)         |
|                      | Chemotherapy | 0.31 (0.23, 0.383)      | 0.337 (0.237, 0.48)                | 0.132 (0.053, 0.263)         | 0.344 (0.218, 0.429)     |

Table 2: Parameter estimates for treatment and control arms in the EMPOWER study (mean and 95% confidence intervals).

## 7 Proofs

**Proposition 1.** Let  $\mathbf{C}$  be a  $k$ -dimensional lower triangular matrix,  $\mathbf{X} = \mathbf{C}\mathbf{C}^T$ , then

$$\frac{\partial \text{vech}(\mathbf{X})}{\partial \text{vech}(\mathbf{C})} = \mathbf{L}_k [(\mathbf{C} \otimes \mathbf{I}) + (\mathbf{I} \otimes \mathbf{C})\mathbf{K}_k] \mathbf{T}_k \mathbf{D}_k,$$

where  $\mathbf{D}_k$  and  $\mathbf{L}_k$  are duplication and elimination matrix separately. And  $\mathbf{K}_k$  is the commutation matrix.  $\mathbf{T}_k$  is a  $k^2 \times k^2$  sparse matrix with 1 in position  $(j, j)$  ( $j \in \{1, 2, \dots, k, k+2, k+3, \dots, 2k, 2k+3, 2k+4, \dots, 3k, \dots, k^2\}$ ) and 0 elsewhere.

*Proof.*

$$d\mathbf{X} = d\mathbf{C}\mathbf{C}^T + \mathbf{C}d\mathbf{C}^T.$$

$$\text{vec}(d\mathbf{X}) = (\mathbf{C} \otimes \mathbf{I}) \text{vec}(d\mathbf{C}) + (\mathbf{I} \otimes \mathbf{C}) \text{vec}(d\mathbf{C}^T).$$

$$\text{vec}(d\mathbf{X}) = ((\mathbf{C} \otimes \mathbf{I}) + (\mathbf{I} \otimes \mathbf{C})\mathbf{K}_k) \text{vec}(d\mathbf{C}).$$

$$\mathbf{L}_k \text{vec}(d\mathbf{X}) = \mathbf{L}_k [(\mathbf{C} \otimes \mathbf{I}) + (\mathbf{I} \otimes \mathbf{C})\mathbf{K}_k] \mathbf{T}_k \mathbf{D}_k \text{vech}(d\mathbf{C}).$$

$$\text{vech}(d\mathbf{X}) = \mathbf{L}_k [(\mathbf{C} \otimes \mathbf{I}) + (\mathbf{I} \otimes \mathbf{C})\mathbf{K}_k] \mathbf{T}_k \mathbf{D}_k \text{vech}(d\mathbf{C}).$$

And this ends the proof.  $\square$

**Proposition 2.**  $\forall$  measurable functions  $h_1$ ,  $h_2$  and  $h_3$ , we have

$$\begin{aligned} & E[h_1(t_i^*) \cdot h_2(\omega_i) \cdot h_3(\mathbf{b}_i)|t_i^*, \mathbf{y}_i, \Delta_i = 0] \\ &= \frac{\int_0^{e_i^*} h_1(t_i^*) \cdot h_2(\omega_i) E[h_3(\mathbf{b}_i)|\mathbf{y}_i, \omega_i, \Delta_i = 0] f(\mathbf{y}_i|\omega_i, \Delta_i = 0) f(\omega_i|t_i^*, \Delta_i = 0) d\omega_i}{\int_0^{e_i^*} f(\mathbf{y}_i|\omega_i, \Delta_i = 0) f(\omega_i|t_i^*, \Delta_i = 0) d\omega_i}, \end{aligned}$$

and

$$\begin{aligned} & E[h_1(t_i^*) \cdot h_2(\omega_i) \cdot h_3(\mathbf{b}_i)|t_i^* > t_i, \mathbf{y}_i, \Delta_i = 0] \\ &= \frac{\int_{t_i}^{\infty} \int_0^{e_i^*} h_1(t_i^*) \cdot h_2(\omega_i) E[h_3(\mathbf{b}_i)|\omega_i, \mathbf{y}_i, \Delta_i = 0] f(\mathbf{y}_i|\omega_i, \Delta_i = 0) f(\omega_i|t_i^*, \Delta_i = 0) f(t_i^*|\Delta_i = 0) d\omega_i dt_i^*}{\int_{t_i}^{\infty} \int_0^{e_i^*} f(\mathbf{y}_i|\omega_i, \Delta_i = 0) f(\omega_i|t_i^*, \Delta_i = 0) f(t_i^*|\Delta_i = 0) d\omega_i dt_i^*}, \end{aligned}$$

*Proof.*

$$\begin{aligned} & E[h_1(t_i^*) \cdot h_2(\omega_i) \cdot h_3(\mathbf{b}_i)|t_i^*, \mathbf{y}_i, \Delta_i = 0] \\ &= E[E[h_1(t_i^*) \cdot h_2(\omega_i) \cdot h_3(\mathbf{b}_i)|t_i^*, \mathbf{y}_i, \omega_i, \Delta_i = 0]] \\ &= \int_0^{e_i^*} h_1(t_i^*) \cdot h_2(\omega_i) E[h_3(\mathbf{b}_i)|t_i^*, \mathbf{y}_i, \omega_i, \Delta_i = 0] f(\omega_i|t_i^*, \mathbf{y}_i, \Delta_i = 0) d\omega_i \\ &= \frac{1}{f(\mathbf{y}_i|t_i^*, \Delta_i = 0)} \int_0^{e_i^*} h_1(t_i^*) \cdot h_2(\omega_i) E[h_3(\mathbf{b}_i)|t_i^*, \mathbf{y}_i, \omega_i, \Delta_i = 0] f(\omega_i, \mathbf{y}_i|t_i^*, \Delta_i = 0) d\omega_i \\ &= \frac{\int_0^{e_i^*} h_1(t_i^*) \cdot h_2(\omega_i) E[h_3(\mathbf{b}_i)|\mathbf{y}_i, \omega_i, \Delta_i = 0] f(\mathbf{y}_i|\omega_i, \Delta_i = 0) f(\omega_i|t_i^*, \Delta_i = 0) d\omega_i}{\int_0^{e_i^*} f(\mathbf{y}_i|\omega_i, \Delta_i = 0) f(\omega_i|t_i^*, \Delta_i = 0) d\omega_i}. \end{aligned}$$

$$\begin{aligned}
& E[h_1(t_i^*) \cdot h_2(\omega_i) \cdot h_3(\mathbf{b}_i)|t_i^* > t_i, \mathbf{y}_i, \Delta_i = 0] \\
&= \int_{t_i}^{\infty} E[h_1(t_i^*) \cdot h_2(\omega_i) \cdot h_3(\mathbf{b}_i)|t_i^*, \mathbf{y}_i, \Delta_i = 0] f(t_i^*|\mathbf{y}_i, t_i^* > t_i, \Delta_i = 0) dt_i^* \\
&= \int_{t_i}^{\infty} E[E[h_1(t_i^*) \cdot h_2(\omega_i) \cdot h_3(\mathbf{b}_i)|t_i^*, \mathbf{y}_i, \omega_i, \Delta_i = 0]] \frac{f(t_i^*, \mathbf{y}_i, t_i^* > t_i, \Delta_i = 0)}{f(\mathbf{y}_i, t_i^* > t_i, \Delta_i = 0)} dt_i^* \\
&= \int_{t_i}^{\infty} \int_0^{e^{t_i^*}} h_1(t_i^*) \cdot h_2(\omega_i) E[h_3(\mathbf{b}_i)|t_i^*, \mathbf{y}_i, \omega_i, \Delta_i = 0] f(\omega_i|t_i^*, \mathbf{y}_i, \Delta_i = 0) d\omega_i \frac{f(t_i^*, \mathbf{y}_i, \Delta_i = 0)}{f(\mathbf{y}_i, t_i^* > t_i, \Delta_i = 0)} dt_i^* \\
&= \frac{1}{f(\mathbf{y}_i, t_i^* > t_i, \Delta_i = 0)} \int_{t_i}^{\infty} \int_0^{e^{t_i^*}} h_1(t_i^*) \cdot h_2(\omega_i) E[h_3(\mathbf{b}_i)|t_i^*, \mathbf{y}_i, \omega_i, \Delta_i = 0] f(\omega_i, \mathbf{y}_i, t_i^*, \Delta_i = 0) d\omega_i dt_i^* \\
&= \frac{\int_{t_i}^{\infty} \int_0^{e^{t_i^*}} h_1(t_i^*) \cdot h_2(\omega_i) E[h_3(\mathbf{b}_i)|\omega_i, \mathbf{y}_i, \Delta_i = 0] f(\mathbf{y}_i|\omega_i, \Delta_i = 0) f(\omega_i|t_i^*, \Delta_i = 0) f(t_i^*|\Delta_i = 0) d\omega_i dt_i^*}{\int_{t_i}^{\infty} \int_0^{e^{t_i^*}} f(\mathbf{y}_i|\omega_i, \Delta_i = 0) f(\omega_i|t_i^*, \Delta_i = 0) f(t_i^*|\Delta_i = 0) d\omega_i dt_i^*}.
\end{aligned}$$

□

## References

- [Alt et al., 2025] Alt, E. M., Qu, Y., Damone, E. M., Liu, J.-o., Wang, C., and Ibrahim, J. G. (2025). Jointly modeling time-to-event and longitudinal data with individual-specific change points: A case study in modeling tumor burden. *Statistics in Medicine*, 44(5):e70021.
